# Supplementary material for: SNED: Superposition Network Architecture Search for Efficient Video Diffusion Model
Source: arXiv:2406.00195 source file (2024-05-31)
Supplement: Supplementary file 1 [file X_suppl.tex]

\clearpage
\setcounter{page}{1}
\maketitlesupplementary

\setcounter{equation}{0}
\setcounter{figure}{0}
\setcounter{table}{0}
\makeatletter

\appendix

Supplementary material provides more details of the experiment results, which include 
% 1) the matrix score evaluation of the pixel-space video diffusion base model; 
1) other used optimization strategies including exponential Moving Average (EMA) strategy and image-based diffusion model transfer learning method; 
and 2) the visualization of the pixel-space video diffusion model spatial super-resolution results according to different model sizes and different resolution choices.

We include the second part's generated videos in the supplementary material package. And show the comparison of them with an HTML file. Please unzip the package and open the HTML file for better visualization. 

\section{Other Optimization Strategies}

To achieve a better and faster NAS training performance, we also conduct a systematic fast training optimization strategy integrating EMA training strategy and image-based diffusion model transfer learning method.

For the EMA training strategy. We begin by training the supernet using standard training procedures, where architecture weights are updated in each iteration. However, in parallel, we maintain an EMA model. After each training iteration, we update the parameters of the EMA model. EMA is calculated by exponentially smoothing the weights of the supernet. This smoothing process assigns a higher weight to the most recent parameter updates while gradually diminishing the influence of past updates. During the architecture evaluation phase, instead of using the most recent weights from the supernet, we use the EMA model's weights. This provides a more stable and consistent representation of the architecture's performance. 

To leverage the image-text datasets that are significantly larger and more diverse than available video-text datasets, we first train a large image diffusion model, and then transfer it to our video diffusion model's supernet. We achieve this model transfer by adding additional temporal blocks into each diffusion block inside the image diffusion model.

\section{Pixel-space Video Diffusion Model Super-resolution Results Visualization}

We also show the pixel-space video diffusion model spatial super-resolution results according to different model sizes and different resolution choices. For a better visualization, we add this part to the supplementary material with an HTML file. Please unzip the supplementary package, then open the HTML file to directly watch the generated videos. Each video has a total number of 24 frames.

On the HTML page, we show the results come from 3 resolution options (64$\times$64, 128$\times$128, 256$\times$256) with 4 different spatial super-resolution (SSR) model sizes (55\%, 70\%, 85\%, and 100\% compared with the supernet). The number of parameters of the supernet model of SSR is 428M. The corresponding input texts are shown below each group of videos.

From the displayed videos, we can see that all the options in terms of different resolutions and different model sizes achieve consistent video generation results.

% \rev{Modify the visualization of Super-resolution results in the future.}

% \begin{figure*}[h]
%     \centering
%     \includegraphics[width=0.95 \textwidth]{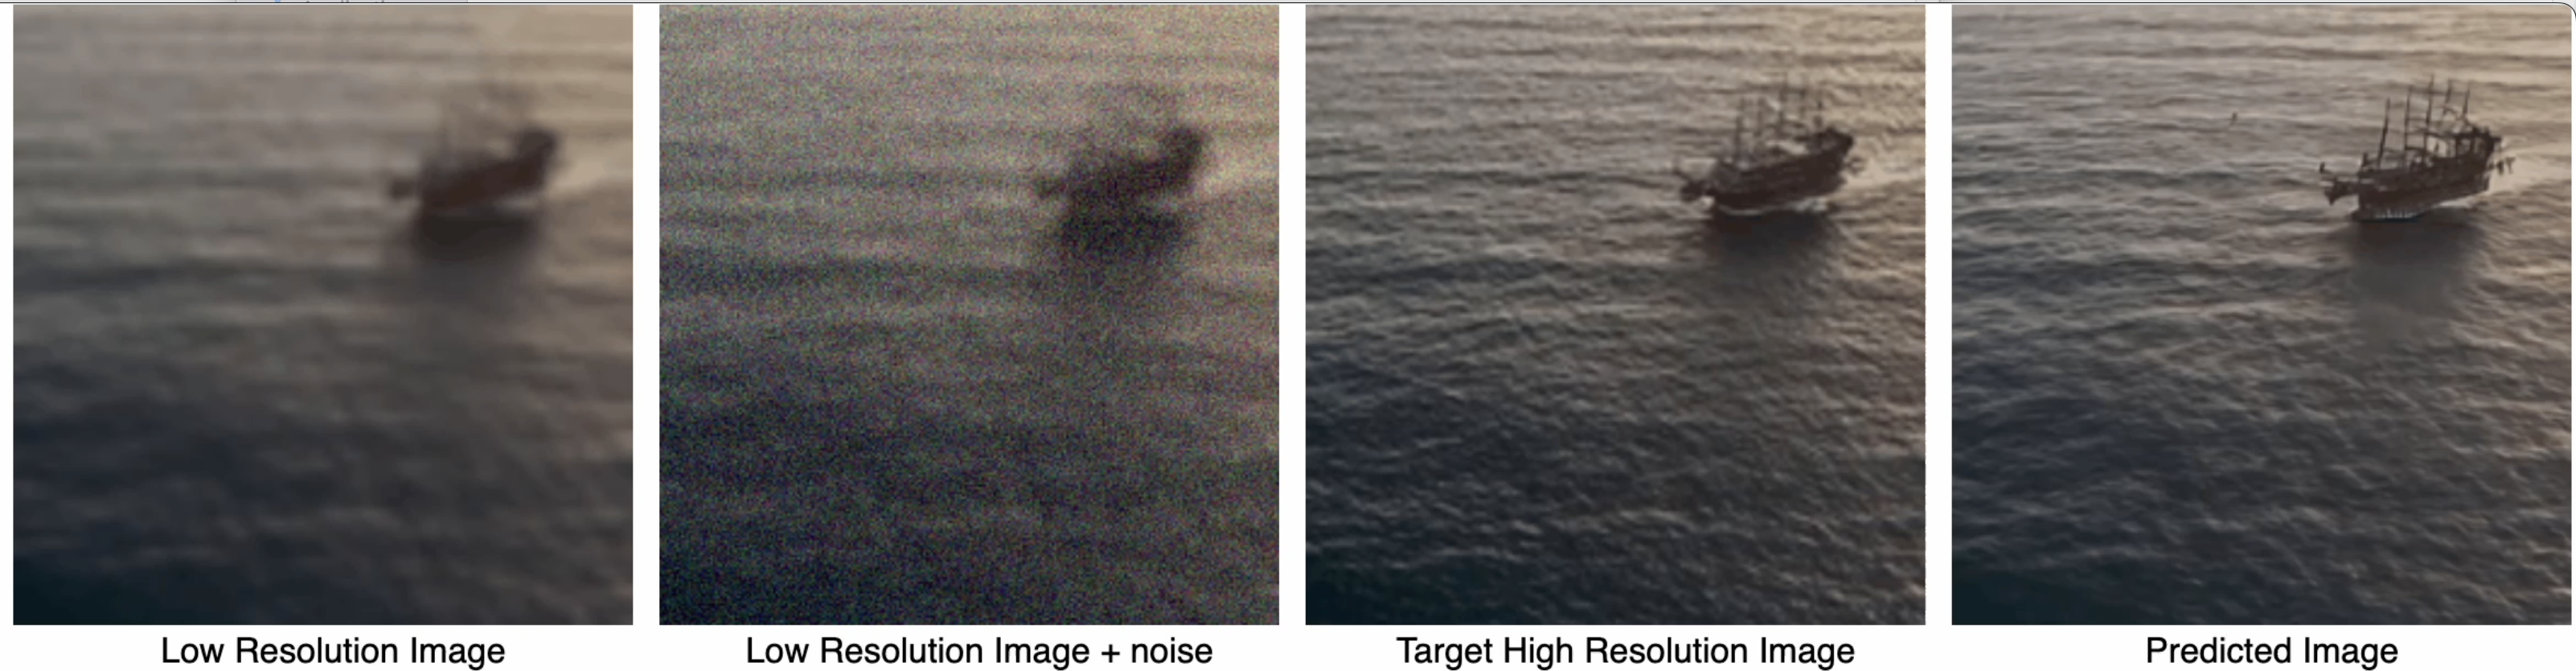}
%     % \vspace{-2mm}
%     \caption{Vertical video of a pirate ship with tourists sailing in the sea.}
%     % \vspace{-2mm}
%     \label{fig:accuracy_gpu}
% \end{figure*}

% \begin{figure*}[h]
%     \centering
%     \includegraphics[width=0.95 \textwidth]{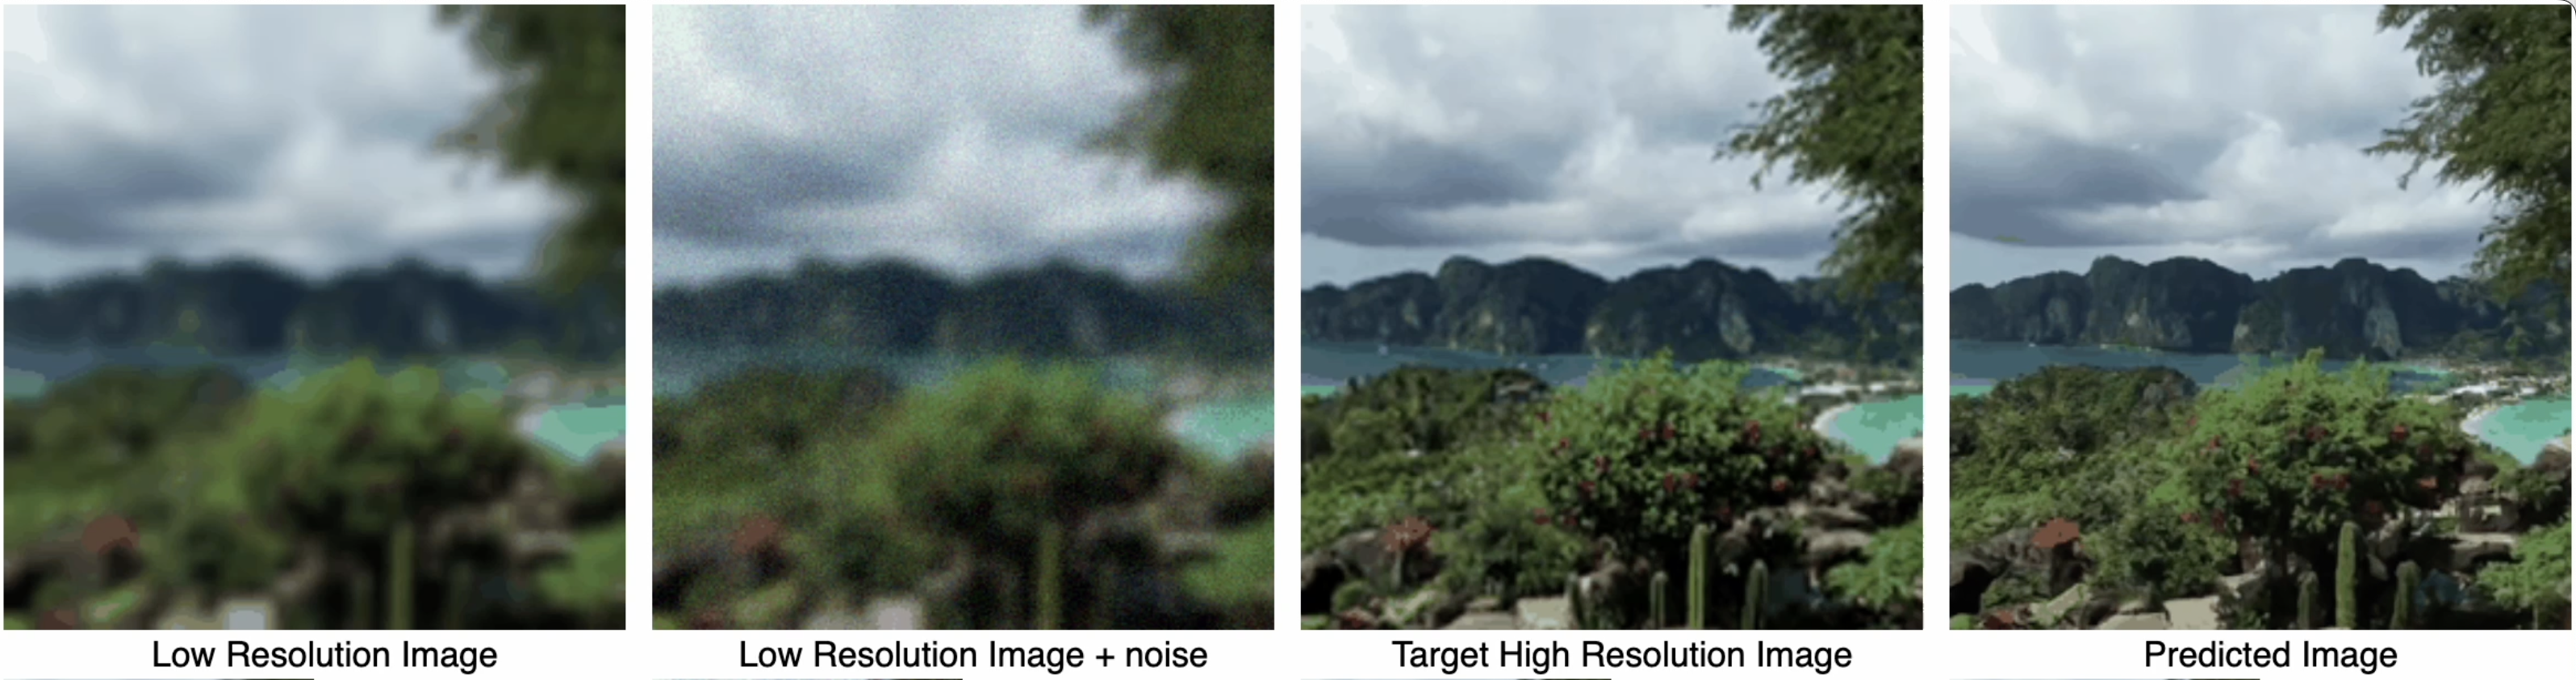}
%     % \vspace{-2mm}
%     \caption{Amazing 4K Drone Video in Koh Phi Phi Thailand.}
%     % \vspace{-2mm}
%     \label{fig:accuracy_gpu}
% \end{figure*}

% \begin{figure*}[h]
%     \centering
%     \includegraphics[width=0.95 \textwidth]{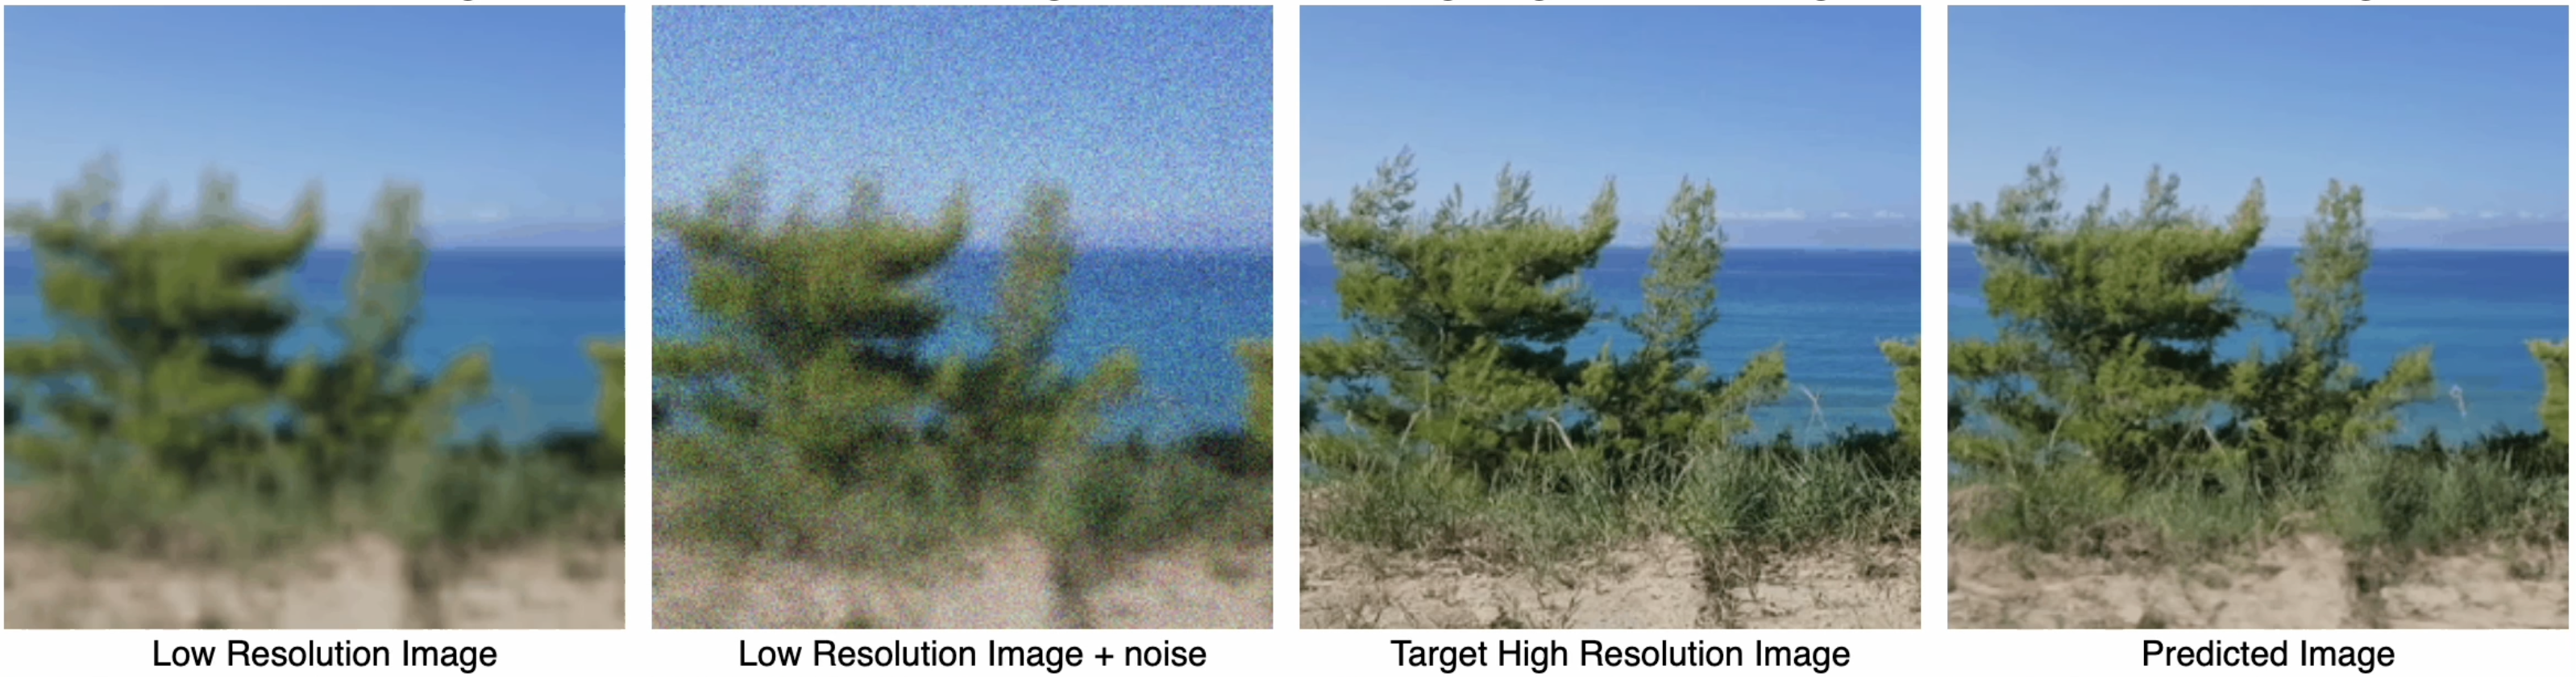}
%     % \vspace{-2mm}
%     \caption{View from the top of the cliff on the endless blue ocean.}
%     % \vspace{-2mm}
%     \label{fig:accuracy_gpu}
% \end{figure*}
